# Supplementary material for: GeoFusion: Geometric Consistency informed Scene Estimation in Dense Clutter
Source: arXiv:2003.12610 source file (2020-09-07)
Supplement: Supplementary file 1 [file appendix.tex]

By using geometric based method, we can find many contact feature pair candidates in a scene. However, not all candidates can be used in optimizations. Because there are still many false contact inference in this way. For example, if two cubes are placed parallel and close to each other on the table, we can detect a P2P contact between these two objects. But there is a chance that those objects are just near to each other but not contacting each other. To avoid those false contact judgment, we add two more physical checks for those contact feature pair candidates. The main idea is that we only consider those contact relationship resulted from gravity, which in other word, those support relationship.

\begin{paragraph}{Support direction check}
If a plane feature wants to support another plane or be supported, its normal direction can not be horizontal. Assume the direction of gravity is $N_G$. The support direction check of plane feature $i$ is as follows:
\begin{equation}
    N_G \cdot N_p^i > \epsilon_G
\end{equation}
where $\epsilon_G$ is the threshold for support direction check.
\end{paragraph}

\begin{paragraph}{Qualitative Support projection check}
If two features have a support relationship, their 2d projection along the direction of gravity must be overlapped. For those contact feature candidates, their 2d projection is the polygon or line projected from their boundary points. Separate axis theorem (SAT) is applied to check the overlap status of those 2d figures. Those feature candidates whose 2d projection is not overlapped with each other will be removed.
\end{paragraph}

\subsection{Geometry Relation Analysis}
Fig. \ref{fig:geometry_relation_compare} compares the results of two optimization stage of the scene in Fig. \ref{fig:teaser}. Left figure is the result of optimization stage I without geometric relation constraints and the right figure is the result after optimized over geometric constraints. The geometric constraints pulled objects to satisfy the constraints. For example, the objects on the right are more aligned with the table and the intersection between objects are fixed. 

\subsection{Detailed Run Time Analysis}
Fig. \ref{fig:time_plot} shows the detailed time analysis with our method. As we are performing stage II optimization every 10th keyframe, the run time at that frame is higher than other frames. In total, the average run time is even lower than 10ms.
